# Supplementary material for: On the complexity of logistic regression models
Source: arXiv:1903.00386 ancillary file (2019-03-01)
Supplement: Supplementary file 1 [file supplementary.pdf]

Supplemental information to:

# "On the complexity of logistic regression models"

**Nicola Bulso[1], Matteo Marsili[2], Yasser Roudi[1]**
[1]The Kavli Institute for Systems Neuroscience and Centre for Neural Computation, NTNU, Trondheim, Norway.
[2]The Abdus Salam International Centre for Theoretical Physics (ICTP), Trieste, Italy.

## 1 Monte Carlo simulations

We report in this section some details of the Monte Carlo simulations that we have performed for evaluating the complexity, namely the integral $e^C = \int d\boldsymbol{\theta} \sqrt{\det F(\boldsymbol{\theta})}$.

Generally, a Monte Carlo method estimates the integral as an average of the values that the integrand takes at random points in the domain. In order to improve the accuracy of the approximation and speed up the convergence, we implemented an importance sampling procedure which allows one to sample the integration space conveniently, weighting more the regions that are carrying out most of the information about the integral. Thus the Monte Carlo estimate of the complexity $e^C = \int d\boldsymbol{\theta} \sqrt{\det F(\boldsymbol{\theta})}$ writes as follows

$$e^C \simeq \frac{1}{N} \sum_{k=1}^{N} \sqrt{\frac{\det F(\boldsymbol{\theta}^{(k)})}{\rho^2(\boldsymbol{\theta}^{(k)})}} \tag{1}$$

where $\rho(\boldsymbol{\theta})$ is a probability distribution, i.e. $\int d\boldsymbol{\theta}\, \rho(\boldsymbol{\theta}) = 1$, and defines the importance sampling procedure.

First of all, we make a change of variable in order to restrict the integration domain to a finite volume. For this purpose we exploit the following relation:

$$\cosh(\boldsymbol{\theta} \cdot \mathbf{x}) = \prod_{k=1}^{n} \cosh(\theta_k) \left\{ \frac{1}{2} \prod_{k=1}^{n} [1 + x_k \tanh(\theta_k)] + \frac{1}{2} \prod_{k=1}^{n} [1 - x_k \tanh(\theta_k)] \right\}. \tag{2}$$

Using the above equation, we can write the elements of the Fisher Information matrix in terms of the new variables $\phi_k = \tanh(\theta_k)$, $\forall k$, which are defined in the finite interval $\phi_k \in (-1, 1)$. With this change of variable the integral becomes $e^C = \int d\boldsymbol{\phi} \prod_{k=1}^{n} (1 - \phi_k^2)^{-1} \sqrt{\det F(\boldsymbol{\theta}(\boldsymbol{\phi}))}$ and by using formula 2 and the definition

of the Fisher Information matrix elements (see main text), we obtain the following expression

$$e^C = \int d\boldsymbol{\phi} \sqrt{\det \tilde{F}(\boldsymbol{\phi}) \prod_{k=1}^{n} (1-\phi_k^2)^{n-2}} \tag{3}$$

where

$$\tilde{F}_{ij}(\boldsymbol{\phi}) = \sum_{\boldsymbol{\mu}} \nu(\boldsymbol{x}^\mu) \frac{4x_i^\mu x_j^\mu}{\left[\prod_{k=1}^n (1+x_k^\mu \phi_k) + \prod_{k=1}^n (1-x_k^\mu \phi_k)\right]^2}. \tag{4}$$

The value of the integral depends on the input distribution $\nu(\mathbf{x})$ through equation 4. Given that the integral is now defined in a finite interval, we can apply the Monte Carlo procedure outlined in equation 1.

If the parameters were all independent the square root of the determinant of the Fisher Information matrix would have been proportional to the product of inverse hyperbolic cosines. We have exploited this fact for defining a family of important sampling functions $\rho(\boldsymbol{\theta}) \propto \prod_{i=1}^n \cosh^{-\gamma}(\theta_i)$ that we have employed for estimating the integral. The case of independent parameters corresponds to the choice $\gamma = 1$, but we have tested the results also with other values of $\gamma$. Given the change of variables $\phi_k = \tanh(\theta_k)$, the importance sampling function becomes $\rho(\boldsymbol{\theta}(\boldsymbol{\phi})) \propto \prod_{i=1}^n (1-\phi_k^2)^{\gamma/2}$. The integral can therefore be evaluated as

$$e^C = \int_{-1}^{1} d\boldsymbol{\phi}\, Q_2(\boldsymbol{\phi}) = (\mathcal{N}_\gamma)^n \int_{-1}^{1} d\boldsymbol{\phi} \tilde{\rho}(\boldsymbol{\phi})\, Q_\gamma(\boldsymbol{\phi}) \simeq (\mathcal{N}_\gamma)^n \frac{1}{N} \sum_{k=1}^{N} Q_\gamma(\boldsymbol{\phi}^{(k)}) \tag{5}$$

where

$$Q_\gamma(\boldsymbol{\phi}) = \sqrt{\det \tilde{F}(\boldsymbol{\phi}) \prod_{i=1}^{n} (1-\phi_i^2)^{n-\gamma}} \tag{6}$$

with $k = 1, ..., N$ sampled i.i.d from the distribution $\tilde{\rho}(\phi_i) = \frac{1}{\mathcal{N}_\gamma}(1-\phi_i^2)^{\frac{\gamma}{2}-1}$, $\forall i$, and $\mathcal{N}_\gamma$ being the normalisation factor. We calculated the integral employing three different sampling procedure: $\gamma = 0.5, 1$ and $2$. The corresponding distributions are shown in Figure 1 (left inset). The sampling from the above mentioned distributions have been obtained as follows

- for $\gamma = 2$, $\mathcal{N}_\gamma = 2$ and $\phi_i$ sampled uniformly in the interval $[-1, 1]$, i.e. $\phi_i \in \mathcal{U}[-1, 1]$, $\forall i = 1, .., n$;
- for $\gamma = 1$, $\mathcal{N}_\gamma = \pi$ and $\phi_i = \sin(w_i)$ with $w_i \in \mathcal{U}[-\pi/2, \pi/2]$, $\forall i = 1, .., n$;
- for $\gamma = 0.5$, $\mathcal{N}_\gamma = 4\mathrm{E}_1(\pi/4, 2)$ and $\phi_i = \sqrt{2}\mathrm{sn}(\sqrt{2}w_i, 0.5)\mathrm{dn}(\sqrt{2}w_i, 0.5)$ with $w_i \in \mathcal{U}[-\mathrm{E}_1(\pi/4, 2), \mathrm{E}_1(\pi/4, 2)]$, $\forall i = 1, .., n$ (here $\mathrm{E}_1(\theta, m)$ is the incomplete elliptic integral of the first kind; $\mathrm{sn}(\theta, m)$ and $\mathrm{dn}(\theta, m)$ are the Jacobi elliptic functions).

Notice that for $\gamma \leq 0$ the density $\tilde{\rho}(\phi)$ is not integrable and for $\gamma > 2$ we would weight more the central region (which is not the one conveying the biggest contribution to the integral) so the right interval should be between 0 and 2. The

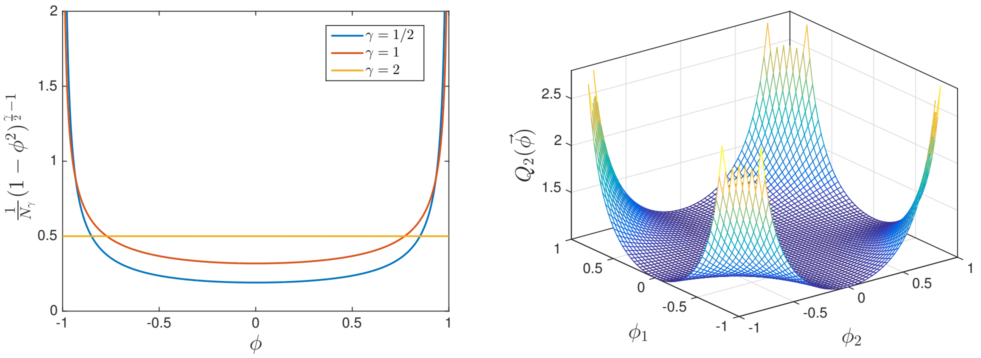


Figure 1: Three different importance sampling schemes employed for evaluating the stochastic complexity (left inset); integrand function in 3 for $n = 2$ (right inset).

function $Q_2(\boldsymbol{\phi})$, which is the integrand in equation 3, is plotted in Figure 1 (right inset) for the case $n = 2$. As we can see in this case, the function varies less in the central region inside the inscribed circle or radius 1 and reaches high values while approaching the vertices. Furthermore we observed the same behaviour also at higher dimensions: we studied the integrand $Q_2(\boldsymbol{\phi})$ as a function of the module of its argument for all values of $n$ between 1 and 10 and we saw that when $1 < |\boldsymbol{\phi}| < \sqrt{n}$ the function exhibits strong oscillations whereas when $|\boldsymbol{\phi}| < 1$ it is almost constant as in the simple two dimensional case in Figure 1 (right inset).

We discuss here the differences in the estimation of the complexity at varying the choice of the candidate function. For this purpose, we report the outcomes of the Monte Carlo integration in the case of uniformly distributed configurations of inputs (which corresponds to the upper bound as described in the section 2 in the paper) at varying the value of $\gamma$. Interestingly, up to a critical dimension which is $n = 5$, the results are independent from the candidate function used for the importance sampling, i.e. the choice of $\gamma$, and suggest that the complexity is well approximated by the relation $e^C \simeq \pi^n/n$. After $n = 5$ the results strongly depends on the importance sampling procedure. This effect can be explained by noting that after $n = 5$, the volume of the n-dimensional sphere of radius one, $V(n)$ in the figure, inscribed in the domain of integration which is an hypercube of side two, starts decreasing with $n$ instead of increasing (black dashed line in Figure 2). Therefore as $n$ grows large the whole volume concentrates around the surface of the hypercube where the integrand is a quickly varying function. As a consequence, beyond the critical dimension, the estimate of the integral becomes extremely sensitive to the sampling of the regions around the vertices of the hypercube.

Given the high variability of the integrand for large $n$, the best candidate functions after this critical point is expected to be $\gamma = 2$ which assign a uniform weight over the entire domain of integration and therefore do not make any assumption of the variability of the function on the borders. In fact, $\gamma = 2$ provides robust estimates: the standard deviations over 100 independent estimates obtained with $\gamma = 2$ are definitively smaller that those obtained with the other choices of $\gamma$ (error bars not shown in the figure for reasons of clarity). Moreover, the mean estimates with $\gamma = 2$ for $n > 5$ keep following the trend $e^C \simeq \pi^n/n$ at varying $n$

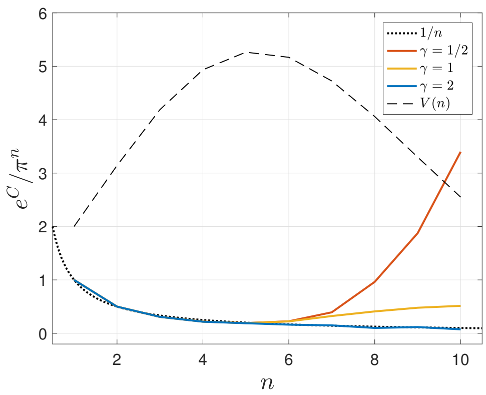


Figure 2: Monte Carlo evaluations of the stochastic complexity $C$ with three different importance sampling schemes. The figure shows that, at least up to a critical dimension $n \approx 5$, the stochastic complexity of a logistic regression model whose input configurations are uniformly distributed can be well approximated by the simple function $e^C = \pi^n/n$. The critical dimension $n \approx 5$ represents the point beyond which the volume of a $n$-dimensional sphere of unitary radius starts decreasing instead of increasing (the trend is depicted in the figure with dashed black line), namely the dimension after which the volume of the domain of integration starts gathering quickly on the surface. Since the integrand is a quickly varying function around the surface of the domain, it follows that, after the aforementioned point, the estimates of the integral will strongly dependent on the importance sampling function. Mean estimates are calculated over 100 independent estimates of the integral, each of which calculated using $10^5$ evaluation of the integrand.

as observed with all candidate function for $n \leq 5$. Finally, the estimates obtained with $\gamma = 0.5$ and $\gamma = 1$ seem to grow larger than $e^C/\pi^n = 1$ which we argued in the main text to be an upper bound for the complexity. Therefore, for all Monte Carlo evaluations we used $\gamma = 2$.

# 2 Motivations for the model selection criteria

We start from an ansatz which could approximatively interpolate between the upper and lower bound for the complexity

$$\log r = -\frac{n}{2}\log\left(\frac{\alpha T H_n}{n}\right) + \log n. \tag{7}$$

As explained in the paper, when $H_n \approx n$, we retrieve the penalisation pertaining models with maximal complexity; whereas when the input distribution is more localised, the resulting penalisation is weaker, especially for large $n$. In fact, in this limit, the factor $T$ is more strongly counterbalanced by $n$, given that $H_n$ is expected to grow as slow as $\log_2 n$.

Therefore, one possible choice of $\alpha$ is $\alpha = \pi/2$ which would match exactly the penalization resulting from the upper bound of the complexity when $H_n \approx n$. However, with this choice, the difference between the upper bound like trend $\log r \sim -\frac{n}{2}\log(\alpha T)$ and the lower bound one $\log r \sim -\frac{n}{2}\log\left(\alpha\frac{TH_N}{n}\right)$ is sometimes very small or not perceptible. This difference can be enhanced by reducing the

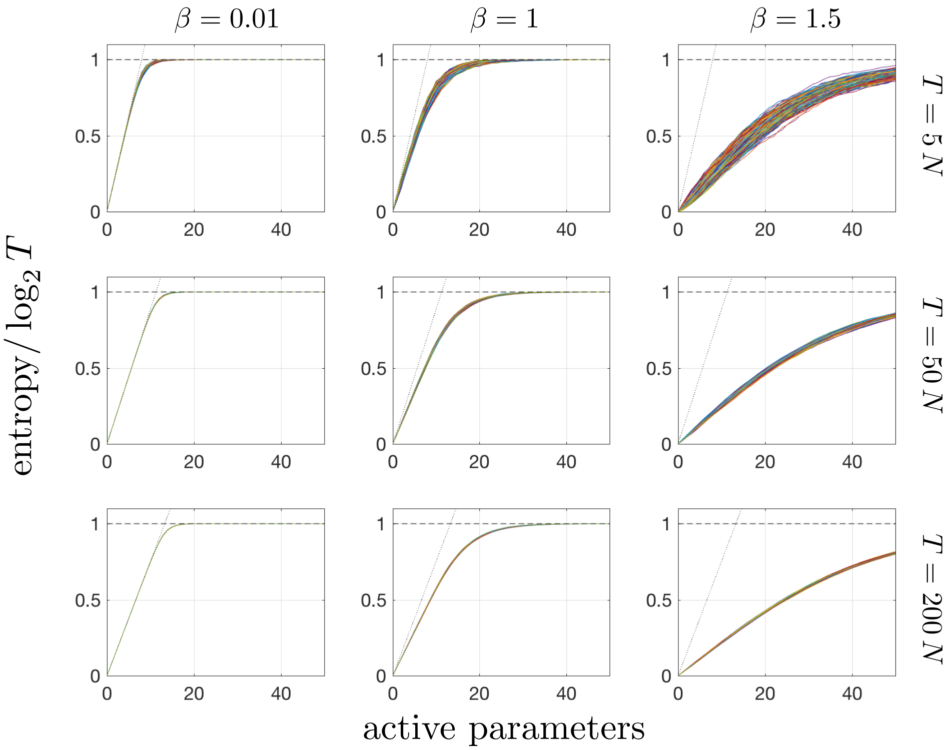


Figure 3: Entropy of input distributions for the subsets of models compared in each numerical test in section 3 plotted against the number of parameters $n$ employed by the models. We report the results at varying the localisation of input distribution $\beta$ (columns) and number of data points $T$ (rows) used in the simulations. In each inset, different lines correspond to 100 independent instances with same $\beta$ and $T$. As explained in the main text, the subset of models compared is obtained by gradually decimating parameters starting from the model with all parameters active. Therefore, in each test we did model comparison on nested models. For small values of $\beta$ the entropy tends to grow linearly with $n$ until reaching the maximal entropy $\log_2 T$. At increasing $\beta$ the rise tends to be slower and almost linear for large $\beta$.

value of $\alpha$. Yet, we need to make sure that the proposed penalisation is a non increasing function of $n$ given that in nested models, the likelihood is a non decreasing function of $n$. Here by nested models we refer to a subset of models for which the model with $n+1$ parameters contains the model with $n$ parameters, for all $n$. Therefore, we require that the first derivative of the penalisation with respect to $n$ is always less or equal than zero. This corresponds of asking that

$$\alpha \geq \frac{n}{TH_n} \exp\left(\frac{2 + n - n^2 {H'}_n/H_n}{n}\right). \tag{8}$$

for any value of $n$, where ${H'}_n$ is the first derivative of the entropy with respect to $n$.

As we can see from Figure 3, the entropy of the input distribution $H_n$ in the simulations performed in the main test (which involved only nested models since we used a decimation approach to walk into the models space) is always a non decreasing function of $n$. The entropy has the largest growth for small models where it tends to grow as $n$ then it bends reaching a plateau corresponding to the

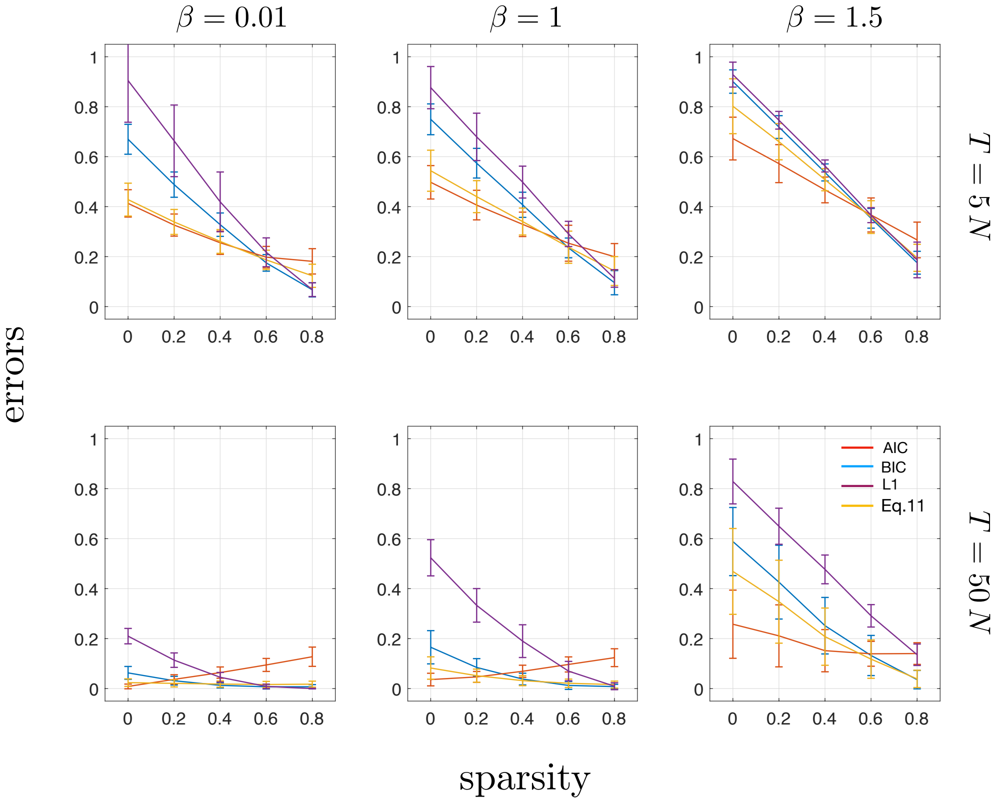


Figure 4: Same numerical simulations as described in the main text (section 3), but the size of the input layer is now $N = 100$. The reconstruction errors versus the sparsity of the ground truth and for different levels of the localisation of input distribution $\beta$ (columns) and sample size T (rows). The errors are the mean fraction of misclassified active/inactive parameters over 100 independent realisations of the same experiments and the error bars are the corresponding standard deviations. We compared performance employing different model selection criteria: AIC (red), BIC (blue), our method, i.e. equation 11 in the main text, (yellow) and logistic regression with l1 regularization (purple).

entropy of the full design matrix. The growth is faster when $\beta$ is small, whereas it becomes slower and almost linear when $\beta$ is large. In both cases, the right hand side of equation 8 is maximised by $\alpha^* = e/H_N$, for any $n$, and choices of $T$ and $N$, provided that when the entropy growth tends to be linear ($\beta > 1$), $T$ is at least as large as $T = e \cdot N$ which is a reasonable requirement given that, as we saw in the main text (section 3), a large dataset is needed in this regime to achieve small reconstruction errors. Therefore, the value $\alpha^* = e/H_N$ represents the optimal value for $\alpha$ such that the penalisation would be maximally affected by the entropy of the input distribution while still being consistently a non increasing function of $n$. By plugging this value into equation 7, we derive our criterion (equation 11 in the main text). We have also tested different choices for $\alpha$, but $\alpha^*$ was always the best compromise in terms of reconstruction error at varying the level of sparsity, e.g. the optimal value at all levels of sparsity.

As we have already shown in the paper with numerical simulations, our proposal performs better than other commonly used model selection recipes. In fact, we saw that with the other investigated methods, the quality of model recovery strongly depends on the sparsity of the ground truth. Instead, our proposal acts against this unbalance trying to deliver the best achievable result at every level of sparsity. In Figure 4, we report additional numerical simulations where we performed the same simulations as in the main text (section 3), but with a different size of the input layer, namely $N = 100$. The simulations further confirm our results and the superiority of the proposed model selection recipe.

# 3 Mapping the 13 keys method into a Bayesian Model selection framework

The dataset of the "13 keys to the White House", that we described in section 4 of the paper, consists of the results of all U.S. presidential elections $w^{(t)}$ and the values of $N = 13$ binary questions (keys) $k_i^{(t)}$ for $i = 1, ..., N$ and $t = 1, ..., T$ (from 1860 to 2016, $T = 40$ elections). The questions are binary, i.e. $k_i^{(t)} \in \{0, 1\}$, and each time the answer is false then $k_i^{(t)} = 1$ (otherwise $k_i^{(t)} = 0$). If six or more keys are false, namely if the sum $K_N^{(t)} = \sum_{i=1}^{N} k_i^{(t)} \geq \delta_N$ with $\delta_N = 6$, then the challenging party is predicted to win the elections, $w^{(t)} = 1$, otherwise the party holding the White House will be more likely to win, $w^{(t)} = 0$. The predictions can be therefore summarized as $w^{(t)} = \Theta(K_N^{(t)} - \delta_N)$ where $\Theta(x)$ is the Heaviside step function, defined as $\Theta(x) = 1$ if $x \geq 0$ and $\Theta(x) = 0$ otherwise, and where, for convenience, we have moved the threshold into the middle of the transition region by subtracting 0.5 from the value of $\delta_N$.

We generalize the 13 Keys method for a generic number of predictor $n \leq N$: $w^{(t)} = \Theta(K_n^{(t)} - \delta_n)$ where $K_n^{(t)}$ is the sum of the $n$ keys belonging to the selection of predictors and $\delta_n$ is the threshold value. The latter depends on $n$ such that $\delta_n = 5.5$ when $n = N$ and $\delta_n = 0.5$ when $n = 1$. A linear interpolation can be used to satisfy the requests: $\delta_n = \text{ceil}((5n + N - 6)/(N - 1)) - 0.5$, $\forall n \geq 1$, where the ceil function approximates the argument to the closest integer greater or equal

than its value.

By transforming the variables $w^{(t)}$ and $k_i^{(t)}$ into the variables $y^{(t)} = 2w^{(t)} - 1$ and $x_i^{(t)} = 2k_i^{(t)} - 1$, the predictions can be equivalently stated as $y^{(t)} = 2\Theta(X_n^{(t)} - b_n) - 1$ with $b_n = 2\delta_n - n$ and $X_n^{(t)} = \sum_i x_i^{(t)}$, where the sum extends to the selection of $n$ predictors.

In the paper we consider the probabilistic counterparts of the above defined deterministic models, namely the 1-parameter degenerate logistic regression models of equation 12 in the paper. In fact in the limit $\theta \gg 1$, the models defined by equation 12 will tend to their deterministic counterparts, i.e. $y = 2\Theta(X_n - b_n) - 1$.

Our goal is to identify the model $\mathcal{M}$, i.e. the subset of predictors, which maximize the posterior probability $p(\mathcal{M}|\hat{X})$ with $X^{(t)} = (\boldsymbol{x}^{(t)}, y^{(t)})$ and $\hat{X} = (X^{(1)}, X^{(2)}, ..., X^{(T)})$ among other candidates. There are $2^N$ ways of selecting $n \leq N$ input indices and therefore, since $N = 13$, our pool of models will be composed of $2^N = 8192$ models. The pool includes also the case $n = 0$ in which none of the predictors are selected and the outcomes of the elections are modelled as completely random events not determined by any of the $N$ predictors. Moreover, considering probabilistic models allows us to exploit a Bayesian Model Selection framework for comparing model and to evaluate their complexity. In the assumption that a priori all models are equally likely and employing a Jeffreys prior for the scalar parameter $\theta$, i.e. $J(\theta) = \sqrt{F(\theta)} / \int d\theta \sqrt{F(\theta)}$, the posterior probability is given by $p(\mathcal{M}|\hat{X}) \propto \int d\theta \exp(T\ell(\theta)) J(\theta)$, where $\ell(\theta)$ is the likelihood function of equation 16 in the paper. As discussed in section 2, the posterior can be approximated by an expansion in $T$: $\log p(\mathcal{M}|\hat{X}) \propto T\ell(\theta^*) - 1/2 \log(T/2\pi) - \log \int d\theta \sqrt{F(\theta)} + O(1/T)$, where $\theta^*$ is the maximum likelihood estimator of the parameter $\theta$. In this case, the BIC penalisation factor does not help discerning among models because it penalize all competing models by the same amount since all models have the same number of parameters. Thus the largest and solely penalisation term which is left in the expansion and which would penalise differently models with the same number of parameters is represented by the complexity term, $C = \log \int d\theta \sqrt{F(\theta)}$.
